# Supplementary material for: Complexity Matters: Dynamics of Feature Learning in the Presence of Spurious Correlations
Source: arXiv:2403.03375 source file (2024-08-24)
Supplement: Supplementary file 1 [file 21_proof.tex]

%auto-ignore
% \section{Analysis of learning dynamics on 2-1 spurious boolean dataset}\label{appendix:proof:dynamics}

% \paragraph{Initalization}. Our initalization is slightly different \citep{glasgow_sgd_2023}. We choose the initalization on the weight to be the scaled version of our previous proof. This allow us to directly applied the previous calculation. And we will also do a straightforward calculation to argue that the weights are 1-well-spread vector per the definition of \citep{glasgow_sgd_2023} which allow us to use their approximation results contained in their Section B directly, 


% \paragraph{Gradient Descent Updates}. For our purpose, GD is enough as our main concern at this time is on the computational complexity or hardness of optimization lies in this problem (it could be very interesting to study how spurious correlation affect sample complexity w.r.t NN for future works).

% \paragraph{Notation}
% For a vector $v, \|v\|$ denote the $l_2$ norm. All asymptotic notation is with respect to $d \to \infty$. $w(1)$ denotes growing to infinity with $d$.

% \paragraph{Case Study: 2-1 Distribution}
% Following the boolean spurious setting, we study the case where the core function is 2-parity $f_c(x) = x_1x_2$ and the spurious function is 1-parity $f_s(x) = x3$. Following \citep{glasgow_sgd_2023}, for a neuron $(a_w,w)$ we decompose $w = w_{1:2} + w_{3} + w_\bot$ or equivalently $w=w_c + w_s + w_\bot$. We further decompose $w_{1:2} = \wcsig + \wcopp$ defined in
% Table~\ref{table:notation}, along with future shorthand we will introduce in this section. We also define \begin{equation*}
%     \mu_1 = e_1 + e_2\;, \mu_2 = e_1 - e_2\; \mu_s = e_3\;
% \end{equation*}
% \begin{table}
%   \caption{Summary of Notation used in Proof Overview and Proofs (core)}
%   \label{table:notation}
%   \centering
%   \begin{tabular}{c|c|c}
%     \toprule
%     $\wcsig = \begin{cases}\frac{1}{2}\mu_1\mu_1^Tw & a_w \geq 0 \\
%     \frac{1}{2}\mu_2\mu_2^Tw & a_w < 0\end{cases}$
%     &
%     $\wcopp = \begin{cases}\frac{1}{2}\mu_2\mu_2^Tw & a_w \geq 0\\
%     \frac{1}{2}\mu_1\mu_1^Tw & a_w < 0\end{cases}$ 
%     &
%     $w_c = \wcsig + \wcopp$      \\
%     \midrule
%     $\wssig = sign(a_w)w_s$ & 
%     $\wsopp = -sign(a_w)w_s$ & 
%  \\
%     \midrule
%     $\begin{cases}
%         \ycmu = f_{\rho}(\mu)y^c(\mu) \\
%         \ysmu = f_{\rho}(\mu)y^s(\mu)
%     \end{cases}$ &
%     $
%     \begin{cases}
%         \ycmin = \min_{\mu \in \{\pm \mu_1, \pm \mu_2\}}\ycmu \\
%         \ysmin = \min_{\mu \in \{\pm \mu_s\}}\ysmu
%     \end{cases}
%     $& $
%     \begin{cases}
%         \ycmax = \max_{\mu \in \{\pm \mu_1, \pm \mu_2\}}\ycmu \\
%         \ysmax = \max_{\mu \in \{\pm \mu_s\}}\ysmu
%     \end{cases}
%     $\\
%     \midrule
%     $\begin{cases}
%         \gmu = |\ell'_{\rho}(\mu)|
%     \end{cases}$ &
%     $\begin{cases}
%         \gcmin = \min_{\mu \in \{\pm \mu_1, \pm \mu_2\}}|\ell'_{\rho}(\mu)|\\
%         \gsmin = \min_{\mu \in \{\pm \mu_s\}}|\ell'_{\rho}(\mu)|
%     \end{cases}$
%      & $\begin{cases}
%          \gcmax = \max_{\mu \in \{\pm \mu_1, \pm \mu_2\}}|\ell'_{\rho}(\mu)| \\
%          \gsmax = \max_{\mu \in \{\pm \mu_s\}}|\ell'_{\rho}(\mu)| 
%      \end{cases}$\\
% \bottomrule
%   \end{tabular}
% \end{table}

% \paragraph{Assumption 1: Clean Gradient}
% We define the clean gradient to be \begin{equation*}
%     \nabla_w^{cl} L_\rho \defeq a_w E_x[\ell'_\rho(z)\drelu(w^Tx)x]
% \end{equation*}
% where $z\defeq x_c+x_s$. We assume \begin{equation*}
%     \nabla_w^{cl} L_\rho \approx \nabla_w L_\rho
% \end{equation*} In simple words, this assumption require the model to has little weights on noisy coordinates or unrelated part of the data. In our setting, this could be show by the fact that gradient of noisy coordinates goes in the opposite direction when weights on core or spurious coordinates are large. 


% \paragraph{Assumption 2: Equal Margin}
% We define $\ycmu \defeq y^c(\mu)\fp(\mu)$ for any $\mu$ in the span of $x_c$ and $\ysmu \defeq y^s(\mu)\fp(\mu)$ for any $\mu$ in the span of $x_s$ We assume \begin{equation*}
%     \ycmax \approx \ycmin \; , \ysmax \approx \ysmin
% \end{equation*}.
% We will use $\yc$ and $\ys$ refer to these two quantites. In simple words, in our setting, this assumption require the model to give approximately equal confidence and accuracy to all correct directions of a parity function, which is reasonable as the distribution we are dealing with is symmetric. In the real world setting, this would require the model to give similar, correct response when presented with positive and negative samples showing only the core or spurious feature.

% \paragraph{Assumption 3: Addition of core and spurious Margin}
% We want argue \begin{equation*}
%     \fp (z) \approx \fp (x_c) + \fp (x_s)
% \end{equation*}
% Note this assumption is valid if the network seperated into two parts as we empirical shown in the experiment section. \citep{kirichenko_last_2023} also observe this empirically with the waterbirds dataset and termed it as "logits additivity". Based on these three assumptions, we derive a general form of population graident for spurious coordinates and core coordinates. 

% \subsection{Population gradient at initialization case study for 2-1 parity.}
% We will give explicit formula for different types of coordinates for population gradient at initialization. The 2-1 population gradient at initalization provides several insights because in this case we know clearly what direction the network is learning. The results for the uniform part is given in \citep{glasgow_sgd_2023} C.Lemma C.4. Here we give the corresponding part for the $\dsame$ distribution.

% \begin{lemma}[Signal Subspace $L_0$ Population Gradients on $D_U$]\label{lemma:pop1}
% For any neuron $(w, a_w)$, we have
% \begin{enumerate}
%     \item \label{Psig} $-\wcsig \nabla_{w} L_0 = \frac{\sqrt{2}}{4}|a_w|\mathbb{E}_{\xi}\mathbf{1}(|w^T\xi| \leq \sqrt{2}\|\wcsig\|)\|\wcsig\|$
%     \item \label{Popp} $-\wcopp \nabla_{w} L_0 = -\frac{\sqrt{2}}{4}|a_w|\mathbb{E}_{\xi}\mathbf{1}(|w^T\xi| \leq \sqrt{2}\|\wcopp\|)\|\wcopp\|$
%     \item \label{Pwpe}  $-\wpe^T\nabla_{w} L_0 = \begin{cases}
%         \frac{|a_w|}{4}\mathbb{E}_{\xi}[\mathbf{1}(|w^T\xi| \in [\sqrt{2}\|\wcsig\|, \sqrt{2}\|\wcopp\|])|w^T\xi|] & \|\wcopp\| > \|\wcsig\|;\\
%       -\frac{|a_w|}{4}\mathbb{E}_{\xi}[\mathbf{1}(|w^T\xi| \in [\sqrt{2}\|\wcopp\|, \sqrt{2}\|\wcsig\|])|w^T\xi|] & \|\wcopp\| \leq \|\wcsig\|.
%     \end{cases}$
%     \item \label{Pwinf} For $i \in [3, d]$, with $X = (\xi - e_i\xi_i)^Tw$, we have $$-w_i\nabla_{w_i} L_0 = \frac{|a_w||w_i|}{4}\left(\mathbb{P}\left[X \in [\sqrt{2}\|\wcopp\| - |w_i|, \sqrt{2}\|\wcopp\| + |w_i|]\right] - \mathbb{P}\left[X \in [\sqrt{2}\|\wcsig\| - |w_i|, \sqrt{2}\|\wcsig\| + |w_i|]\right]\right).$$
% \end{enumerate}
% \end{lemma}

% \begin{lemma}[Signal Subspace $L_0$ Population Gradients on $\dsame$]\label{lemma:pop1}
% For any neuron $(w, a_w)$, we have
% \begin{enumerate}
%     \item \label{Psigdsame} $-\wcsig \nabla_{w} L_0 = \frac{\sqrt{2}}{4}|a_w|\mathbb{E}_{\xi}\mathbf{1}(|\wssig| - \sqrt{2}\|\wcsig\| \leq w^T\xi \leq |\wssig| + \sqrt{2}\|\wcsig\|)\|\wcsig\|$
%     \item \label{Poppdsame} $-\wcopp \nabla_{w} L_0 = -\frac{\sqrt{2}}{4}|a_w|\mathbb{E}_{\xi}\mathbf{1}(|\wssig| - \sqrt{2}\|\wcopp\| \leq w^T\xi \leq |\wssig| + \sqrt{2}\|\wcopp\|)\|\wcopp\|$
%     \item \label{Pwpedsame} $-\wpe^T\nabla_{w} L_0 = \frac{|a_w|}{8}\E_\xi[(\ind(|\wpe \xi| \geq |\sqrt{2}\|\wcsig\| + \wssig|) +\ind(|\wpe \xi| \geq |-\sqrt{2}\|\wcsig\| + \wssig|) -\ind(|\wpe \xi| \geq |\sqrt{2}\|\wcopp\| - \wssig|) -\ind(|\wpe \xi| \geq |\sqrt{2}\|\wcopp\| - \wssig|))|\wpe \xi|]$
%     \item \label{Pwsdsame} $-w_s \nabla_{w} L_0 = \frac{1}{4}|a_w| \wssig \E_{\xe}[\drelu(\sqrt{2}\|\wcsig\| + \wssig + \wpe \xe) + \drelu(-\sqrt{2}\|\wcsig\| + \wssig + \wpe \xe) - \drelu(\sqrt{2}\|\wcopp\| - \wssig + \wpe \xe) - \drelu(-\sqrt{2}\|\wcopp\|- \wssig + \wpe \xe)]$
%     \item \label{Pwinfdsame} For $i \in [4, d]$, with $X = (\xi - e_i\xi_i)^Tw$, we have $-w_i\nabla_{w_i} L_0 = \frac{|a_w||w_i|}{8} \E_{\xe}[\ind(|\sqrt{2}\|\wcsig\| + \wssig + w^T X| \leq |w_i|) + \ind(|-\sqrt{2}\|\wcsig\| + \wssig + w^T X| \leq |w_i|) - \ind(|\sqrt{2}\|\wcopp\| - \wssig + w^T X|\leq |w_i|) - \ind( |-\sqrt{2}\|\wcopp\| - \wssig + w^T X| \leq |w_i|)]$
% \end{enumerate}
% \end{lemma}

% Notice how the $\dsame$ distribution change the expression of the original population gradient. The change is due to that $\dsame$ has a fixed $x_s$ depending on different value of $x_c$

% \subsection{Derivation of Loss formula}
% The goal is to show that the loss of the network is approximately described by a simple formula. For a neuron $(a_w, w)$, we have

% The goal is to show that the loss of the network is approximately described by a simple formula. For a neuron $(a_w, w)$, we have \begin{align*}
%     &-\wcsig \nabla_w L_{\rho_t}  \\
%     \approx& -\wcsig E_x[a_w l'_{\rho_t}(z) \sigma'(w^Tx) x] \tag{Assumption 1}\\
%     =& -\wcsig \left( \lambda E_{x\sim D_{same}}[a_w \ell'(z)\sigma'(w^Tx) x] + (1-\lambda) E_{x\sim D_{diff}}[a_w \ell'(z)\sigma'(w^Tx) x] \right) \\
%     =& 2 \lambda E_{x\sim D_{same}}[a_w y(x)(1-sig(y(x)f_{\rho_t}(x_c) + y(x)f_{\rho_t}(x_s)))\sigma'(w^Tx) \wcsig \cdot x] \\
%     +&2 (1-\lambda) E_{x\sim D_{diff}}[a_w y(x)(1-sig(y(x)f_{\rho_t}(x_c) + y(x)f_{\rho_t}(x_s)))\sigma'(w^Tx) \wcsig \cdot x] \tag{Assumption 3}\\
%     =& 2 \lambda E_{x\sim D_{same}}[a_w y(x)(1-sig(\yc + \ys))\sigma'(w^Tx) \wcsig \cdot x] \\
%     +&2 (1-\lambda)(1-sig(\yc - \ys) E_{x\sim D_{diff}}[a_w y(x)\sigma'(w^Tx) \wcsig \cdot x] \tag{Assumption 2}
% \end{align*}
% Note that through symetrization by flipping $x_c$ (as fliping $x_c$ does not change the label $y^c(x_c)=y^c(-x_c)$. We have for the $D_{same}$ \begin{align*}
%     &E_{x\sim D_{same}}[a_w y(x)(1-sig(\yc + \ys))\drelu(w^Tx) \wcsig \cdot x] \\
%     =&(1-sig(\yc + \ys)) E_{x\sim D_{same}}[a_w y(x_c)\drelu(w_s^Tx_s + w_c^Tx_c + \wpe^Tx_\bot) \wcsig \cdot x_c] \\
%     =&\frac{1}{2}(1-sig(\yc + \ys)) E_{x\sim D_{same}}[a_w y(x_c)(\drelu(w_s^Tx_s + w_c^Tx_c + \wpe^Tx_\bot) - \drelu(w_s^Tx_s - w_c^Tx_c + \wpe^Tx_\bot)) \wcsig \cdot x_c] \\
%     =&\frac{1}{2}(1-sig(\yc + \ys)) E_{x\sim D_{same}}[a_w y(x_c)(\ind(|w_c^Tx_c| \geq |w_sx_s + \wpe^T x_\bot|)sign(w_c^Tx_c) \wcsig \cdot x_c]\\
%     =&\frac{\sqrt{2}}{4} (1-sig(\yc + \ys)) |a_w|E_{x\sim D_{same}}[(\ind(\sqrt{2}\|\wcsig\| \geq |w_sx_s + \wpe^T x_\bot|) \|\wcsig\|]
% \end{align*}
% And similarly for the $D_{diff}$ we have \begin{align*}
%     &E_{x\sim D_{diff}}[a_w y(x)(1-sig(\yc + \ys))\drelu(w^Tx) \wcsig \cdot x] \\
%     =&\frac{\sqrt{2}}{4} (1-sig(\yc - \ys)) |a_w|E_{x\sim D_{diff}}[a_w y(x_c)(\ind(\sqrt{2}\|\wcsig\| \geq |w_sx_s + \wpe^T x_\bot|) \|\wcsig\|]
% \end{align*}
% And in summary we have \begin{align*}
%     & -\wcsig \nabla_w L_{\rho_t} \\
%     \approx & \frac{\sqrt{2}}{2} \lambda (1-sig(\yc + \ys)) |a_w|E_{x_s, x_\bot \sim D_u}[(\ind(\sqrt{2}\|\wcsig\| \geq |w_sx_s + \wpe^T x_\bot|) \|\wcsig\|] \\
%     + & \frac{\sqrt{2}}{2} (1-\lambda) (1-sig(\yc - \ys)) |a_w|E_{x_s, x_\bot \sim D_{u}}[(\ind(\sqrt{2}\|\wcsig\| \geq |w_sx_s + \wpe^T x_\bot|) \|\wcsig\|]
% \end{align*}

% And similarly for $w_s$, using the three assumptions, we have \begin{align*}
%     & -w_s \nabla_{w_s} L_{\rho_t} \\
%      \approx & \frac{1}{2} \lambda (1-sig(\yc + \ys)) a_w w_s E_{x_\bot\sim D_{u}}[\drelu(w_1+w_2+w_s+\wpe x_\bot)
%      + \drelu(-w_1-w_2+w_s+\wpe x_\bot) \\
%      +& \drelu(w_1-w_2-w_s+\wpe x_\bot)
%      + \drelu(-w_1+w_2-w_s+\wpe x_\bot)] \\
%     - & \frac{1}{2} (1-\lambda) (1-sig(\yc - \ys)) a_w w_s E_{x_\bot\sim D_{u}}[\drelu(w_1+w_2-w_s+\wpe x_\bot)
%      + \drelu(-w_1-w_2-w_s+\wpe x_\bot)\\
%      +& \drelu(w_1-w_2+w_s+\wpe x_\bot)
%      + \drelu(-w_1+w_2+w_s+\wpe x_\bot)]
% \end{align*}


% % We will first study the neurons that are heavy in $\|\wcsig\|$ but weak in $\wssig$ at initalization e.g a neuron that has $(a_w = 1, w = [1,1, -1, ...])$. Thus $\|\wcsig\| = \sqrt{2}\theta$ and $\wssig=-\theta$. We will assume $d$ be large here. For a vector $u \in {\pm \theta}^d$. By the Berry-Essen inequality we have $P_{\xi \sim {\pm 1}}[u^T \xi \geq x] \approx P[G \geq \frac{x}{\sqrt{d}\theta}]$, where $G$ is a standard gaussian R.V. Note that by our initalization and gradient descent $u$ always satisfy the requirement. We use $\Phi(a,b) \defeq P_G[G \in [a,b]]$ and $\Phi(a) \defeq P_G[G \leq a]$ 

% % \begin{enumerate}
% %     \item  $-\wcsig \nabla_{w} L_0 = \frac{\theta^2 }{2} \Phi(-\frac{1}{\sqrt{d}}, \frac{3}{\sqrt{d}})$
% %     \item  $-\wcopp \nabla_{w} L_0 = 0$
% %     \item  For $i \in [4, d]$, with $X = (\xi - e_i\xi_i)^Tw$, we have $-w_i\nabla_{w_i} L_0 = \frac{\theta^2}{8} (\Phi(\frac{2}{\sqrt{d}},\frac{4}{\sqrt{d}}) - \Phi(\frac{0}{\sqrt{d}},\frac{2}{\sqrt{d}})) $
% %     \item $-w_s \nabla_{w} L_0 = \frac{\theta^2}{4}\Phi(-\frac{1}{\sqrt{d}}, \frac{3}{\sqrt{d}})$
% % \end{enumerate}

% % Now for neurons heavy in $\wssig$ but weak in $\|\wcsig\|$ i.e $(a_w=1, w=[1,-1, 1])$. We have
% % \begin{enumerate}
% %     \item  $-\wcsig \nabla_{w} L_0 = 0$
% %     \item  $-\wcopp \nabla_{w} L_0 = -\frac{\theta^2 }{2} \Phi(-\frac{1}{\sqrt{d}}, \frac{3}{\sqrt{d}})$
% %     \item  For $i \in [4, d]$, with $X = (\xi - e_i\xi_i)^Tw$, we have $-w_i\nabla_{w_i} L_0 = \frac{\theta^2}{8} (\Phi(\frac{0}{\sqrt{d}},\frac{2}{\sqrt{d}}) - \Phi(\frac{2}{\sqrt{d}},\frac{4}{\sqrt{d}})) $
% %     \item $-w_s \nabla_{w} L_0 = \frac{\theta^2}{4}\Phi(-\frac{1}{\sqrt{d}}, \frac{3}{\sqrt{d}})$
% % \end{enumerate}

% % For neurons heavy in both $\wssig$ and $\|\wcsig\|$ i.e $(a_w=1, w=[1,1,1])$. We have \begin{enumerate}
% %     \item  $-\wcsig \nabla_{w} L_0 = \frac{\theta^2 }{2} \Phi(-\frac{1}{\sqrt{d}}, \frac{3}{\sqrt{d}})$
% %     \item  $-\wcopp \nabla_{w} L_0 = 0$
% %     \item  For $i \in [4, d]$, with $X = (\xi - e_i\xi_i)^Tw$, we have $-w_i\nabla_{w_i} L_0 = \frac{\theta^2}{8} (\Phi(\frac{2}{\sqrt{d}},\frac{4}{\sqrt{d}}) - \Phi(\frac{-1}{\sqrt{d}},\frac{1}{\sqrt{d}})) $
% %     \item $-w_s \nabla_{w} L_0 = \frac{\theta^2}{4}\Phi(-\frac{1}{\sqrt{d}}, \frac{3}{\sqrt{d}})$
% % \end{enumerate}

% % For neurons that is weak in both $\wssig$ and $\|\wcsig\|$ i.e $(a_w = 1, w=[1,-1,-1])$. We have \begin{enumerate}
% %     \item  $-\wcsig \nabla_{w} L_0 = 0$
% %     \item  $-\wcopp \nabla_{w} L_0 = -\frac{\theta^2 }{2} \Phi(-\frac{1}{\sqrt{d}}, \frac{3}{\sqrt{d}})$
% %     \item  For $i \in [4, d]$, with $X = (\xi - e_i\xi_i)^Tw$, we have $-w_i\nabla_{w_i} L_0 = \frac{\theta^2}{8} (\Phi(\frac{0}{\sqrt{d}},\frac{2}{\sqrt{d}}) - \Phi(\frac{2}{\sqrt{d}},\frac{4}{\sqrt{d}})) $
% %     \item $-w_s \nabla_{w} L_0 = \frac{\theta^2}{4}\Phi(-\frac{1}{\sqrt{d}}, \frac{3}{\sqrt{d}})$
% % \end{enumerate}
